# Supplementary material for: Expected Grad-CAM: Towards gradient faithfulness
Source: arXiv:2406.01274 source file (2024-06-25)

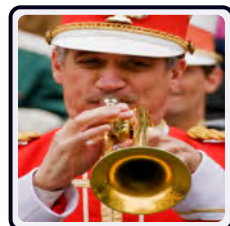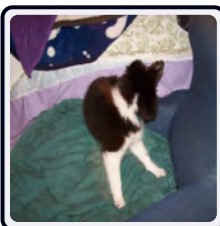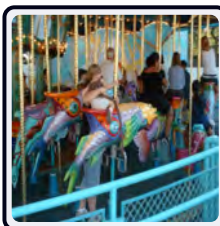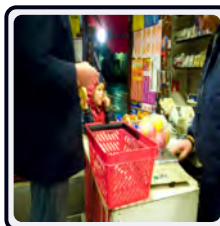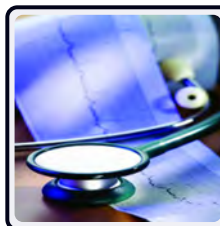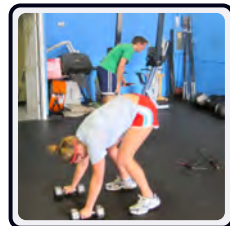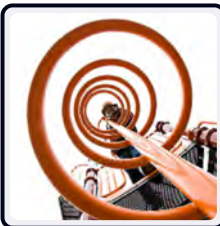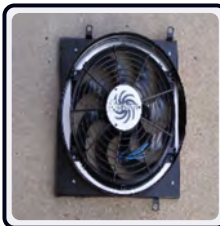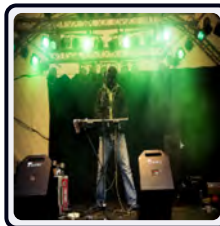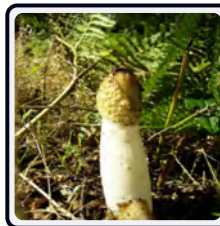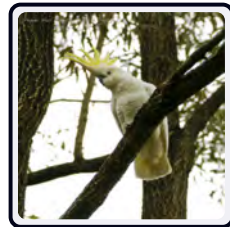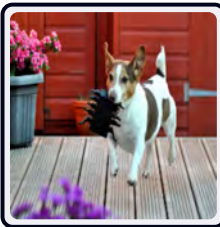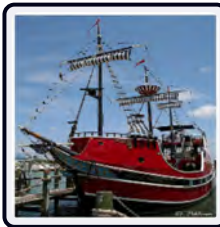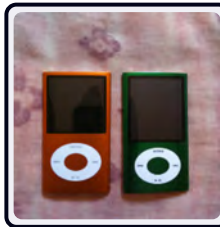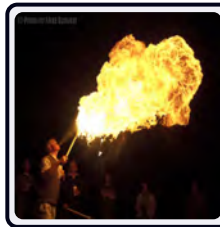

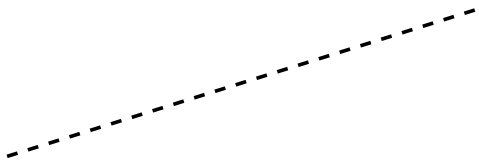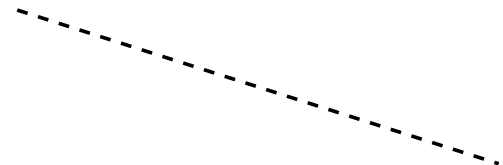

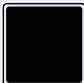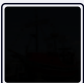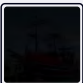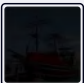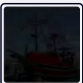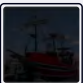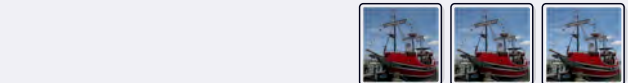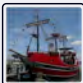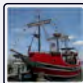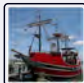

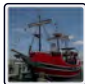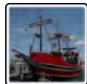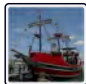

Supplement: Supplementary file 1 [file supp-saturation-samples.pdf]
